# Supplementary material for: Parental Guidance: Efficient Lifelong Learning through Evolutionary Distillation
Source: arXiv:2503.18531 source file (2025-03-24)
Supplement: Supplementary file 1 [file 09_appendix.tex]

% \rmsnote{Assume the reviewer only reads this section. Be self-contained.}

% \textbf{What is the problem?} A clear description of the problem being solved.
% Don't start with something long winded like "It is well known that robotics is a hard problem, blah blah".
% Start with "We focus on the problem of ... (\figref{fig:best})."

% Octi:

% We focus on the problem of developing robotic agents capable of generalizing across diverse environments while maintaining varied behaviors. The main challenge is twofold: first, ensuring that agents can solve a range of difficult tasks; and second, fostering the emergence of diverse solutions to complex problems without converging to a single, monotonic behavior. This challenge is similar to the quality diversity problem, but with a crucial distinction: rather than seeking diversity across multiple policies, we aim to maximize the behavioral expressiveness within a single policy. This allows for greater adaptability and versatility within the agent itself, enabling it to handle diverse environments through a unified approach.


% \textbf{Why is it interesting?} Good place to use an example and draw out the nuances of the problem.

% Octi:

% This problem is particularly interesting when viewed through the lens of natural behavior. In nature, individual organisms adjust their behaviors based on the terrain they encounter. For example, mountain goats navigate steep, rocky slopes by using precise hoof placements and balancing techniques, while on flatter ground, they switch to faster, more energy-efficient movement. Similarly, coyotes alter their movement strategies depending on the terrain—running swiftly in open fields, but relying on stealth and shorter bursts of speed in dense forests or rough, uneven terrain. These adaptations allow the same species to manage different terrains effectively, showcasing a remarkable ability to adapt their movement and behavior without needing external guidance or pre-designed strategies.

% In contrast, artificial systems often struggle to replicate this level of environment-conditioned adaptability. When faced with diverse environments, many current approaches converge on narrow, repetitive strategies, limiting their ability to generalize. Unlike in nature, where organisms dynamically adjust their behavior based on their surroundings, artificial agents often require extensive human intervention, such as style encoding, to adapt across different landscapes and tasks.


% \textbf{Why is it hard?} Describe what other have done [general problem is NP], approximations and assumptions they have made, and how they might be limiting [do it politely].

% Octi:

% For the quality challenge, common approaches include dense rewards and curriculum learning, which guide the agent step-by-step to achieve success. While effective for solving some difficult tasks, these methods often require manual curriculum design and reward shaping for each task, making them difficult to scale. To address the limited expressiveness of policy behaviors, researchers have employed techniques like motion style imitation, which relies on pre-collected datasets of behaviors, or carefully crafted reward and command structures to guide agents toward specific behaviors. These behaviors are then distilled into a diversified policy. Although these methods can be successful, they are labor-intensive, dependent on predefined goals, and require intricate rewards. Moreover, such datasets are primarily available for human-like morphologies, limiting scalability to other morphologies.

% Quality Diversity (QD) algorithms, while promoting behavioral diversity, face limitations in consolidating these behaviors into a unified framework for multi-task agents. They explore diverse solutions but often lack mechanisms to integrate these behaviors into a single, expressive, environment-aware policy. Additionally, QD methods depend on manually defined behavior descriptors, which are difficult to generalize across tasks.

% \textbf{What is our insight?} What are we doing that others did not? Always have one and only one \emph{key insight}. Our key insight is:

% Octi:

% Our key insight is that reproduction—a fundamental and intuitive aspect of natural evolution—can be leveraged to merge and diversify behaviors within a single agent using imitation learning techniques, enabling adaptability across varied tasks. While reinforcement learning (RL) is effective at producing specialized agents for specific terrains, it often falls short when it comes to fostering behavioral diversity. On the other hand, imitation learning consolidates controllers effectively but struggles with adaptability across diverse tasks. Evolutionary methods, especially population-based strategies, have enabled RL to tackle more complex tasks through mutation and survival of the fittest. Quality Diversity (QD) algorithms promote diversity among policies, yet few have explored reproduction as a mechanism for blending behaviors within a single agent. Despite its obvious role in natural evolution, reproduction remains underutilized in artificial evolution approaches. We believe incorporating reproduction into RL can drive the development of more flexible, adaptive agents capable of navigating diverse environments.


% \textbf{What did we do?} Spill the beans (\figref{fig:summary}). 

% \textbf{Contributions.} We make the following contributions:

% \textbf{Limitations.} Weave future work into limitations. 

% \begin{figure}[!t]
% % Always try to place the figure on top of a column to save space
% \centering
% % Use linewidth to adjust width
% % Use textheight(the total height of the column of text) to adjust height
% %\includegraphics[width=\linewidth]{figs/XXX.jpg}
% \framebox[\linewidth]{\raisebox{0pt}[\linewidth][0pt]{{\LARGE The wow figure.}}}
% \caption{Your best figure}
% \label{fig:best}
% \end{figure}
% \newpage
% \begin{figure*}[!t]
% % Always try to place the figure on top of a column to save space
% \centering
% % Use linewidth to adjust width
% % Use textheight(the total height of the column of text) to adjust height
% %\includegraphics[width=\linewidth]{figs/XXX.jpg}
% \framebox[\linewidth]{{\LARGE Explain the entire paper in one figure.}}
% \caption{Your summary figure}
% \label{fig:summary}
% \end{figure*}


% Traditional distillation methods focus on transferring an expert actor's policy into a student actor's policy, aiming to enhance the student's behavioral diversity. While this approach works, it also implies that no further learning occurs after distillation, and the student policy cannot surpass the teacher's performance in its specialized terrain. Our method ensures that the student learns both the actor and critic functions from the expert, and then continues reinforcement learning after this transfer. This allows the student to not only outperform the teacher in their areas of expertise but also become more diversified through ongoing learning.

% \section{Useful resources}
% \begin{enumerate}
%     \item Sandy Kaplan @ UW for grammatical and style proof-reading!
% \end{enumerate}

% \section{Style notes}
% \label{sec:style}
% \begin{enumerate}
% 	\item First person active voice. Always.
% 	\item Make very very pretty figures and tables.
% 	\item Use \textsf{booktabs} for tables and RTFM.
% 	\item Use \textsf{caption} for subfigures and RTFM.
% 	\item Include lots of references (30-40).
% 	\item Be precise with everything.
% 	\item Begin new sections at the top of a page.
% 	\item Write code to make figures. Add data files to repo.
% 	\item Use alg defs like \guild .
% \end{enumerate}

% \textbf{Challenges in Curriculum Learning}
% Curriculum Learning gradually trains agents with increasingly complex tasks, offering a structured way to guide behavior. When done correctly, with a well-designed progression from easy to hard, it achieves remarkable success \citep{rudin2022advanced} \citep{rudin2022learning}. However, these methods are sensitive to learning pitfalls, making the curriculum design resource-intensive to ensure stable and continuous learning, which limits their scalability across diverse and dynamic tasks.

% Coevolution strategies, such as the POET algorithm \citep{wang2019paired}, offer a more hands-free, evolution-based approach that leverages the curriculum method while becoming robust to discontinuities in learning. Instead of relying on manual tuning, coevolution uses evolutionary search to evolve both agents and their environments simultaneously. It maintains a repertoire of capable agents, ensuring that when one fails, progress is not lost, and new agents with different backgrounds can step in and retry. Our work utilize terrain generator \citep{miki2024learning} extends this approach, enabling agents and terrains to co-evolve in more complex 3D environments.
